# Supplementary material for: Lipschitz standardization for multivariate learning
Source: arXiv:2002.11369 source file (2020-10-21)
Supplement: Supplementary file 2 [file discrete.tex]

\documentclass{standalone}

\usepackage{tikz}
\usetikzlibrary{positioning, fit, arrows.meta}

\input{../../macros.tex}

\begin{document}
    \begin{tikzpicture}[
    	dot/.style={circle,fill,inner sep=0.5pt},
    	ft/.style={circle, draw, minimum width=8mm, inner sep=1pt},
    	filter/.style={circle, draw, minimum width=7mm, inner sep=1pt, path picture={\draw[thick, rounded corners, blue] (path picture bounding box.center)--++(65:2mm)--++(0:1mm);
    			\draw[thick, rounded corners, blue] (path picture bounding box.center)--++(245:2mm)--++(180:1mm);}},
    	mylabel/.style={font=\scriptsize\sffamily},
    	]

    	\node[] (x) at (0,0) {$\xb_d\longrightarrow\overline{\xb}_d\longrightarrow\xtildeb_d$};
    	\node[below=1ex of x] (eta) {$\etab_d\longleftarrow\overline{\etab}_d\longleftarrow\etatildeb_d$};

        \draw[orange, ->] (x.east) .. controls (1.8, -0.2) and (1.8, -0.6) .. node[anchor=south, rotate=-90] {\tiny learning} (eta.east);

        \draw[blue, ->] (eta.west) .. controls (-1.8, -0.6) and (-1.8, -0.2)  .. node[anchor=south, rotate=90] {\tiny evaluation} (x.west);
    \end{tikzpicture}
\end{document}
